# Supplementary material for: Are EEG Sequences Time Series? EEG Classification with Time Series Models and Joint Subject Training
Source: arXiv:2404.06966 source file (2026-10-22)
Supplement: Supplementary file 1 [file appendix.tex]

\documentclass[runningheads]{llncs}
\usepackage[T1]{fontenc}
\usepackage{graphicx}
\usepackage{amsfonts}
\usepackage{amsmath}
\usepackage{amssymb}
\usepackage{svg}
\usepackage{mathtools}
\usepackage{booktabs}
\usepackage{cleveref}
\usepackage{multirow}
\usepackage{todonotes}
\usepackage{makecell} % TODO: check if it is not interfering with any other package. Diego addition for table style.
\usepackage{newclude}
\usepackage[misc]{ifsym}

% N.B.: do not change anything above this line. If you require additional packages, please load them directly after this line.
\usepackage{mwe}
% N.B.: you may delete the preceding line. It is used to display an example image in this template.

\begin{document}

\section{Appendix}
In this section, we break down our results for the three datasets MI in \cref{tab:performanceMI}, SSVEP in \cref{tab:performanceSSVEP}, and ERN in \cref{tab:performanceERN} in detail. Here, we list the performance of the Inception, ResNet, and MAtt architecture on a per-subject basis.  

\begin{table}[htbp]
\centering
\caption{Performance Comparison on the MI dataset for the subject-specific case. We report the average accuracy over 5 runs respectively.}
\label{tab:performanceMI}
\begin{tabular}{lccc}
\toprule
\textbf{Subject} & \textbf{Inception} & \textbf{ResNet} & \textbf{MAtt} \\
\midrule
1 & $78.96\pm1.82$ & $72.83\pm3.22$ & $\textbf{86.94}\pm1.36$ \\
2 & $41.25\pm2.63$ & $38.12\pm3.27$ & $\textbf{56.94}\pm2.42$ \\
3 & $82.09\pm3.05$ & $70.76\pm3.10$ & $\textbf{88.33}\pm1.17$ \\
4 & $52.43\pm2.40$ & $49.72\pm3.41$ & $\textbf{67.85}\pm3.42$ \\
5 & $38.75\pm3.74$ & $37.50\pm4.51$ & $\textbf{61.32}\pm1.07$ \\
6 & $48.61\pm1.78$ & $44.58\pm4.39$ & $\textbf{52.50}\pm2.52$ \\
7 & $75.99\pm4.51$ & $62.36\pm3.39$ & $\textbf{91.18}\pm0.89$ \\
8 & $74.31\pm3.28$ & $73.68\pm2.54$ & $\textbf{83.06}\pm2.01$ \\
9 & $73.26\pm2.14$ & $72.92\pm2.24$ & $\textbf{81.18}\pm1.06$ \\
\midrule
\textbf{Summary} & 62.85$\pm$3.21& 58.05$\pm$3.68 & \textbf{74.37}$\pm$3.39\\
\bottomrule
\end{tabular}
\end{table}

\begin{table*}[t]
\centering
\caption{Performance Comparison on the SSVEP dataset for the subject-specific case. We report the average accuracy over 5 runs respectively.}
\label{tab:performanceSSVEP}
\begin{tabular}{lccc}
\toprule
\textbf{Subject} & \textbf{Inception} & \textbf{ResNet} & \textbf{MAtt} \\
\midrule
1 & $80.40\pm2.06$ & $56.40\pm3.98$ & $\textbf{81.60}\pm2.87$ \\
2 & $86.60\pm1.62$ & $75.20\pm3.82$ & $\textbf{89.40}\pm1.36$ \\
3 & $\textbf{61.60}\pm3.07$ & $38.20\pm2.64$ & $58.20\pm5.64$ \\
4 & $\textbf{25.00}\pm4.00$ & $20.40\pm4.41$ & $20.60\pm3.88$ \\
5 & $25.00\pm6.72$ & $22.60\pm1.74$ & $\textbf{26.40}\pm4.80$ \\
6 & $\textbf{79.20}\pm1.72$ & $38.20\pm3.92$ & $79.00\pm2.68$ \\
7 & $\textbf{69.20}\pm1.72$ & $42.80\pm2.14$ & $66.00\pm2.19$ \\
8 & $23.60\pm1.74$ & $23.40\pm1.85$ & $\textbf{23.80}\pm2.71$ \\
9 & $79.40\pm2.58$ & $62.40\pm3.20$ & $\textbf{88.20}\pm2.04$ \\
10 & $68.60\pm3.72$ & $35.00\pm3.03$ & $\textbf{70.60}\pm4.54$ \\
11 & $\textbf{91.20}\pm2.48$ & $63.80\pm6.79$ & $90.20\pm1.47$ \\
\midrule
Summary & 62.71$\pm$2.95 & 43.49$\pm$3.41 & \textbf{63.90}$\pm$1.95\\
\bottomrule
\end{tabular}
\end{table*}

\begin{table}[h]
\centering
\caption{Performance Comparison on the ERN dataset for the subject-specific case. We report the average AUC over 5 runs respectively.}
\label{tab:performanceERN}
\begin{tabular}{lccc}
\toprule
\textbf{Subject} & \textbf{Inception} & \textbf{ResNet} & \textbf{MAtt } \\
\midrule
2 & $81.14\pm4.60$ & $74.03\pm3.37$ & $\textbf{81.86}\pm2.56$ \\
6 & $\textbf{90.89}\pm2.02$ & $88.40\pm2.67$ & $68.34\pm1.76$ \\
7 & $83.45\pm6.80$ & $\textbf{85.45}\pm7.05$ & $69.28\pm10.90$ \\
11 & $59.50\pm10.52$ & $55.27\pm9.19$ & $\textbf{70.50}\pm2.66$ \\
12 & $\textbf{74.49}\pm3.67$ & $68.62\pm9.92$ & $60.62\pm4.70$ \\
13 & $56.34\pm2.26$ & $51.15\pm4.16$ & $\textbf{62.92}\pm3.65$ \\
14 & $\textbf{78.96}\pm2.47$ & $75.22\pm3.17$ & $70.42\pm4.80$ \\
16 & $\textbf{56.09}\pm5.53$ & $50.53\pm3.54$ & $55.71\pm2.56$ \\
17 & $79.93\pm3.78$ & $75.93\pm4.20$ & $\textbf{80.60}\pm5.52$ \\
18 & $\textbf{77.40}\pm1.73$ & $72.30\pm1.39$ & $75.11\pm1.42$ \\
20 & $\textbf{65.90}\pm4.96$ & $59.97\pm2.56$ & $57.60\pm8.12$ \\
21 & $\textbf{74.53}\pm6.72$ & $67.95\pm7.76$ & $62.43\pm9.56$ \\
22 & $\textbf{95.87}\pm2.03$ & $95.09\pm0.89$ & $89.33\pm4.28$ \\
23 & $69.85\pm7.00$ & $61.66\pm2.38$ & $\textbf{70.03}\pm5.40$ \\
24 & $\textbf{77.66}\pm1.36$ & $70.88\pm4.60$ & $73.71\pm2.99$ \\
26 & $54.90\pm5.80$ & $54.03\pm4.66$ & $\textbf{60.08}\pm1.92$ \\
\midrule
Summary & \textbf{73.55}$\pm$5.08 & 69.16$\pm$5.16 & 69.28 $\pm$5.31\\
\bottomrule
\end{tabular}
\label{tab:performance}
\end{table}

To evaluate the standard deviation over the runs we use the following equation:
\begin{align*}
 \ell^{(r)} & := \frac{1}{S} \sum_{i=1}^S \ell(y_n, \hat y^{(r)}(x^i))
\\   
  \text{mean}^{\text{runs}} & := \frac{1}{R}\sum_{r=1}^R \ell^{(r)}
\\                        
   \text{stddev}^{\text{runs}}& := (\frac{1}{R-1}\sum_{r=1}^R (\ell^{(r)} - \text{mean}^{\text{runs}})^2)^{\frac{1}{2}}
\end{align*}

Here, $R$ is the total number of runs.

\end{document}
